# Supplementary material for: Video2Sim2Real: Full-Stack Autonomous Dexterous Skill Acquisition from a Single Human Video
Source: arXiv:2606.08828 source file (2026-06-07)
Supplement: Supplementary file 1 [file E_residual_rl_mp.tex]

\section{Residual RL for Sim-to-Real Transfer on Motion-Planning Trajectories}
\label{sec:Residual_RL_4_MP}
In addition to the observations used for single-trajectory tracking (i.e., $
\mathbf{o}_t =
\left[
\bar{\mathbf{q}}^{\mathrm{cur}}_t,\;
\bar{\mathbf{q}}_{t+1},\;
\mathbf{c}_t,\;
\Delta \mathbf{x}_t,\;
\Delta \theta_t
\right],
$), we also condition the observation on additional goal information to mitigate partial observability arising from trajectory divergence. Speficially, we include the initial 3D flow centroid of each trajectory, and the target one, and also the next-time flow centrpoid posiitons.

It should be noted that the training time is comparable to that of replicating a single human trajectory, as finger adaptation remains similar across all trajectories.
